# Supplementary material for: Search for an Anomalous Production of Charged-Current $\nu_e$ Interactions Without Visible Pions Across Multiple Kinematic Observables in MicroBooNE
Source: arXiv:2412.14407 ancillary file (2025-07-14)
Supplement: Supplementary file 1 [file uBooNE_PeLEE_PRL_Supplemental_Material_Submitted.pdf]

# Supplemental material: Search for an Anomalous Production of Charged-Current $\nu_e$ Interactions Without Visible Pions Across Multiple Kinematic Observables in MicroBooNE

The MicroBooNE Collaboration*
(Dated: December 26, 2024)

## I. IMPACT OF THE CRT ON THE SELECTION

To illustrate the impact of the CRT-based cuts, we show in Fig. 1 the prediction and data for the reconstructed neutrino energy distribution from the $1e0p0\pi$ selection after loose preselection cuts have been applied without (Fig. 1a) and with (Fig. 1b) background rejection from the CRT. The CRT is responsible for "vetoing" events with any activity in time with the neutrino interactions that trigger activity in the CRT panels surrounding the MicroBooNE cryostat. This cut is able to remove 60% of cosmic backgrounds, while rejecting only 3% of CC $\nu_e$ interactions. The MicroBooNE CRT system is described in Ref. [1].

In its application to this analysis, the CRT rejection power is somewhat reduced because the dataset analyzed includes data from runs 1 and 2 (when the CRT subsystem was not installed). The original background rejection strategy had to be optimized based on TPC morphology variables only. Still, when added to the $1e0p0\pi$ selection, CRT-based cuts reject an additional 25.4% of the remaining cosmic ray background with a 98.9% efficiency for electron neutrinos.

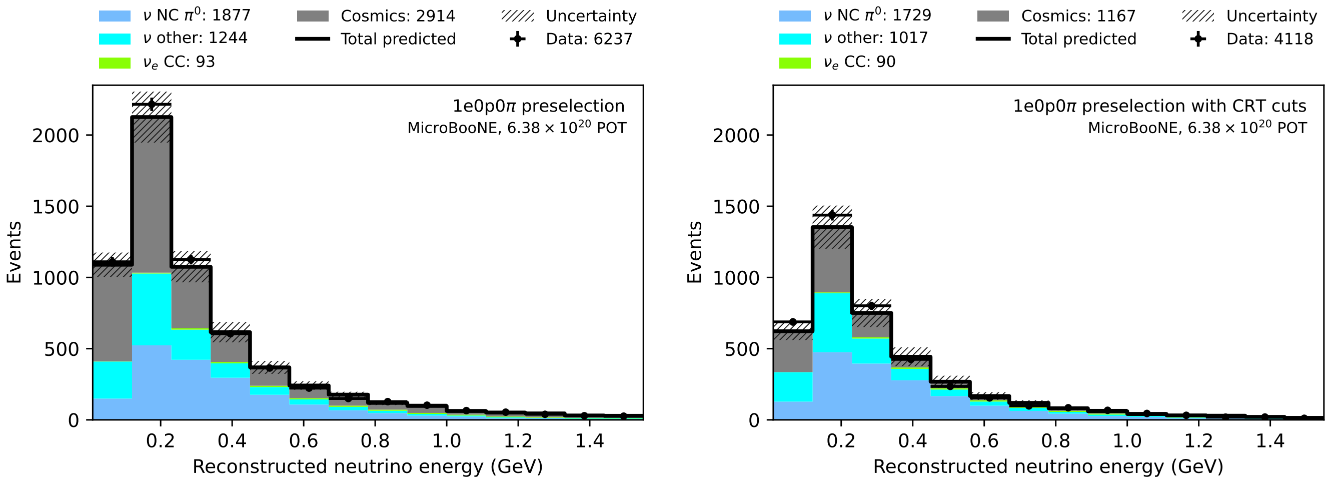


(a) (b)

FIG. 1. Comparison of the prediction and data for the reconstructed neutrino energy distribution from the $1e0p0\pi$ preselection, (a) without and (b) with the application of CRT cuts to the event selection.

## II. CONSTRAINT COVARIANCE AND IMPACT

This analysis leverages several sidebands to constrain both intrinsic $\nu_e$ and NC $\pi^0$ interactions (the leading source of background). The constraint is performed through the conditional constraint formalism in the same way as the first analysis [2]. This constraint procedure relies on the correlations with sideband channels to update the prediction and its uncertainty in the signal region. As a demonstration of the information leveraged by the constraint and the

* microboone_info@fnal.gov

impact it has on the analysis, we show in Fig. 2 the correlation matrix including both signal channels (bottom left 2×2 quadrant) and sideband channels (top right 3×3 quadrant). Fig. 3 then shows the impact the constraint has on the signal prediction for 1$e$N$p$0$\pi$ (Fig. 3a) and 1$e$0$p$0$\pi$ (Fig. 3b) channels. In this figure, the blue solid line and shaded region represents the predicted number of events and 1$\sigma$ uncertainty before the constraint was applied. The analogous information in orange instead shows the constrained prediction and uncertainty. Informed by the data in the sidebands, the central value (CV) slightly shifts in both distributions, and uncertainties generally shrink. The reduction in systematic uncertainty is greater in the 1$e$N$p$0$\pi$ channel compared to the 1$e$0$p$0$\pi$ channel.

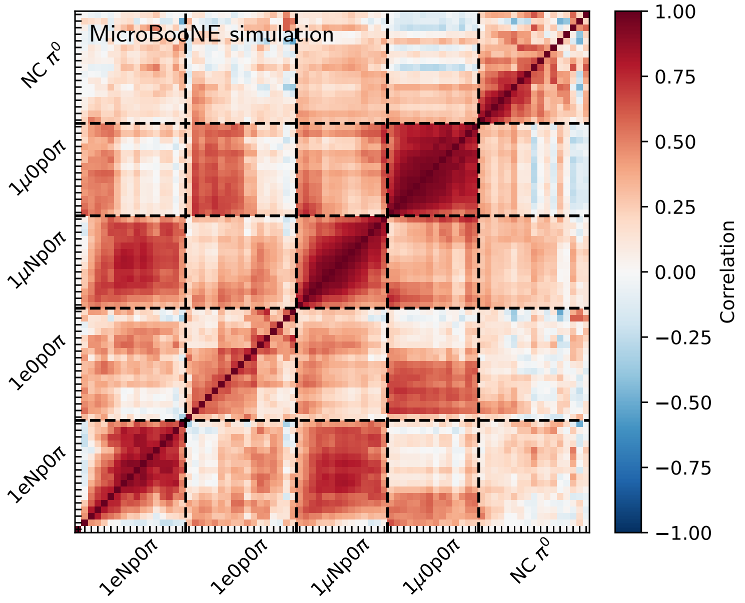


FIG. 2. Correlation matrix between the signal and sideband channels of the analysis. All channels are binned in reconstructed neutrino energy.

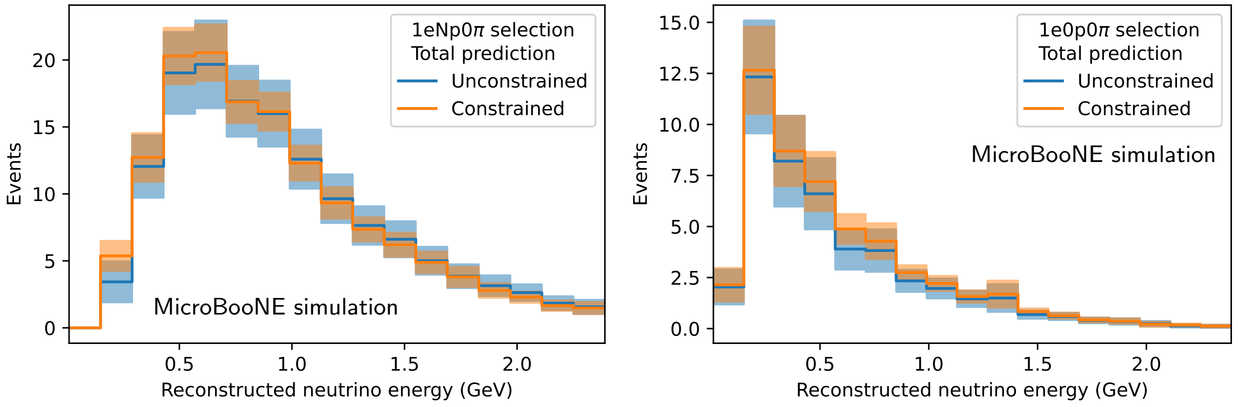


(a) (b)

FIG. 3. MC background predictions (excluding cosmics) in the (a) 1$e$N$p$0$\pi$ and (b) 1$e$0$p$0$\pi$ signal channels with uncertainties, before (blue) and after (orange) applying the constraint procedure.

## III. SMOOTHING OF DETECTOR SYSTEMATICS

Bin-to-bin correlations are sensitive to statistical fluctuations. For detector variation MC samples, this leads to a noisy correlation matrix. To mitigate this issue, we apply a smoothing filter to the histograms of the detector variation

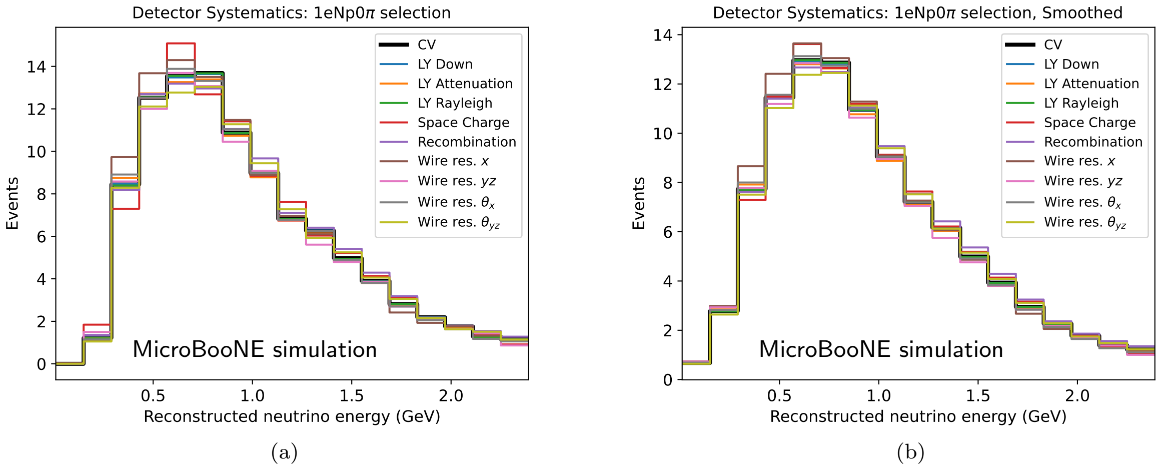


FIG. 4. Detector variation histograms for the $1e\text{N}p0\pi$ signal (a) before and (b) after the application of the smoothing filter. The variations being considered are light yield (LY), space charge and recombination effects, and variations of the wire response.

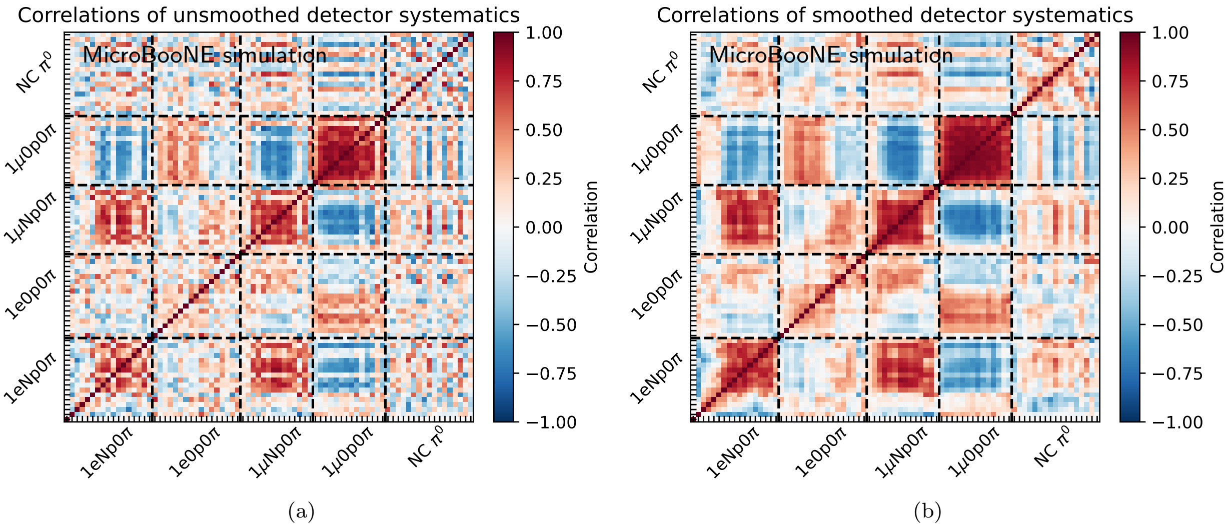


FIG. 5. Correlation matrix of the total detector systematic uncertainty in the signal and control channels (a) before and (b) after the application of the smoothing filter. All channels are binned in reconstructed neutrino energy in the same binning as is used in Figs. 1 and 2 in the Letter.

samples. The filter convolves the bin counts with the normalized weights $F = [0.1, 0.3, 1.0, 0.3, 0.1]/1.8$, meaning that each bin count is replaced by a weighted average of its nearest and next-to-nearest neighbors. The bin counts are extended on both sides by repeating the outermost values two times before applying the filter to reduce edge effects. The result of the smoothing, when applied to the detector variations in the $1e\text{N}p0\pi$ signal selection, is shown in Fig. 4. The correlation matrix resulting from the smoothing is shown in Fig. 5 and shows a good level of noise reduction. This allows us to fully exploit the often sizeable correlations in detector uncertainties, improving the sensitivity of our statistical tests.

## IV. UPDATED SIGNAL MODEL

This section presents details of the *LEE Signal Model 2* built in shower kinematics used in the analysis. While briefly described here, we note that the method by which the signal model is constructed follows the same prescription as documented in Ref. [3] to construct a neutrino-energy-based signal model (*LEE Signal Model 1*) and used for the

first round of the analysis, although now with updated kinematic variables. Both signal models are constructed based on MiniBooNE's neutrino interaction simulation samples. The neutrino-energy-based signal model uses the complete simulation sample, which consists of 72.1% CC events and 29.1% NC events, while the shower-kinematics-based signal model uses only the CC events, as they produce final-state electrons.

The shower-kinematics-based signal model relies on MiniBooNE's efficiency and smearing matrix in shower energy and angle. The smearing matrices for shower energy and angle are shown in Fig. 6. Given the nature of these variables and the uniform angular efficiency and resolution of the MiniBooNE detector, both smearing matrices show strong correlation between the true and reconstructed quantities. The efficiency of MiniBooNE to reconstruct electrons is roughly flat in these variables, averaging 6.1%. While here we present the smearing matrices in one dimension to convey the true-to-reconstructed smearing of each variable, the full two-dimensional efficiency and smearing matrix is used in the unfolding.

The ratio between MiniBooNE's unfolded excess events and the intrinsic electron neutrino events in these variables is used to obtain a scaling of the electron neutrino events in each two-dimensional bin, as shown in Fig. 7. The enhanced rate of $\nu_e$-induced electron events is particularly pronounced in the most forward-going and low-energy bin with enhancement of more than ten times the intrinsic $\nu_e$ rate. Fig. 8 and Fig. 9 show MicroBooNE's truth-level electron energy and $\cos(\theta)$ spectra broken into final-state topology, without any selection cuts applied, for *LEE Signal Model 1* and *2*, respectively. The *LEE Signal Model 2* obtained from the MiniBooNE dataset predicts a visible excess primarily in the range of 150-500 MeV for electron energy and 0.7-1.0 for electron $\cos(\theta)$.

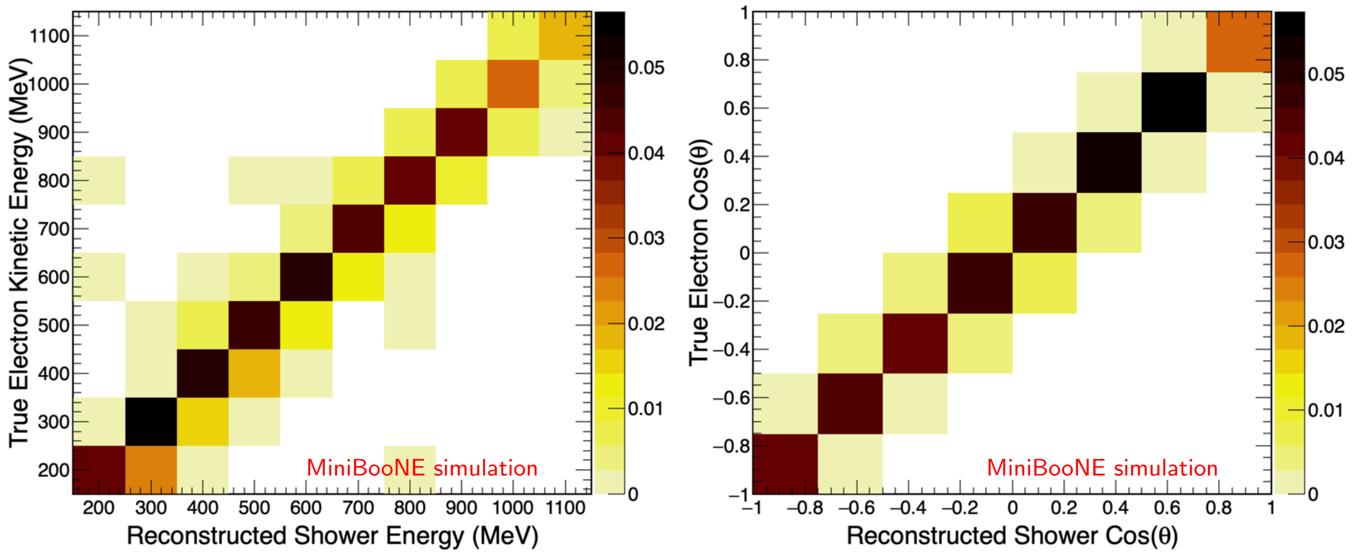


(a)

(b)

FIG. 6. MiniBooNE response matrix for electron shower energy and $\cos(\theta)$.

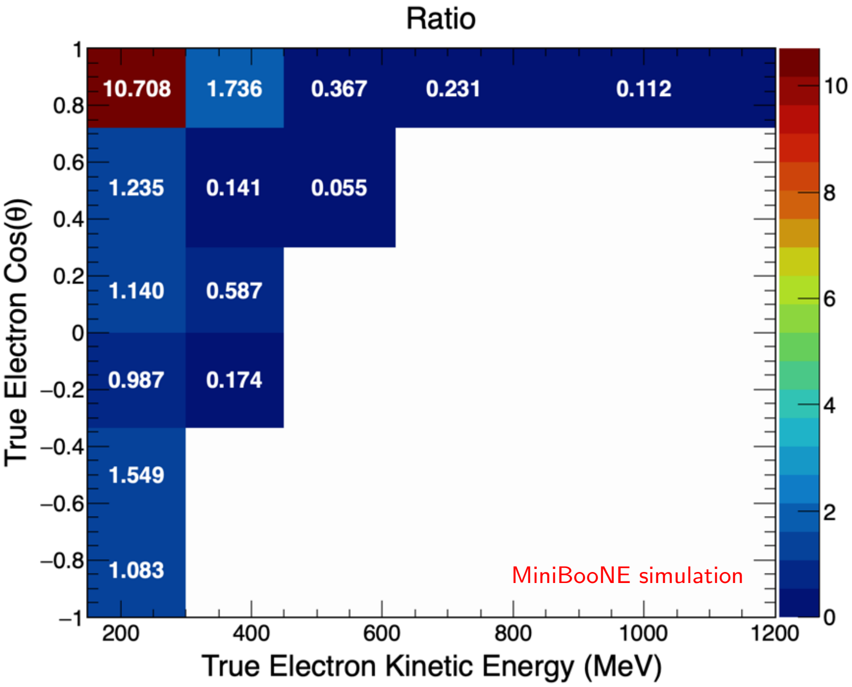


FIG. 7. The LEE ratio model unfolded from MiniBooNE shower two-dimensional kinematic variables.

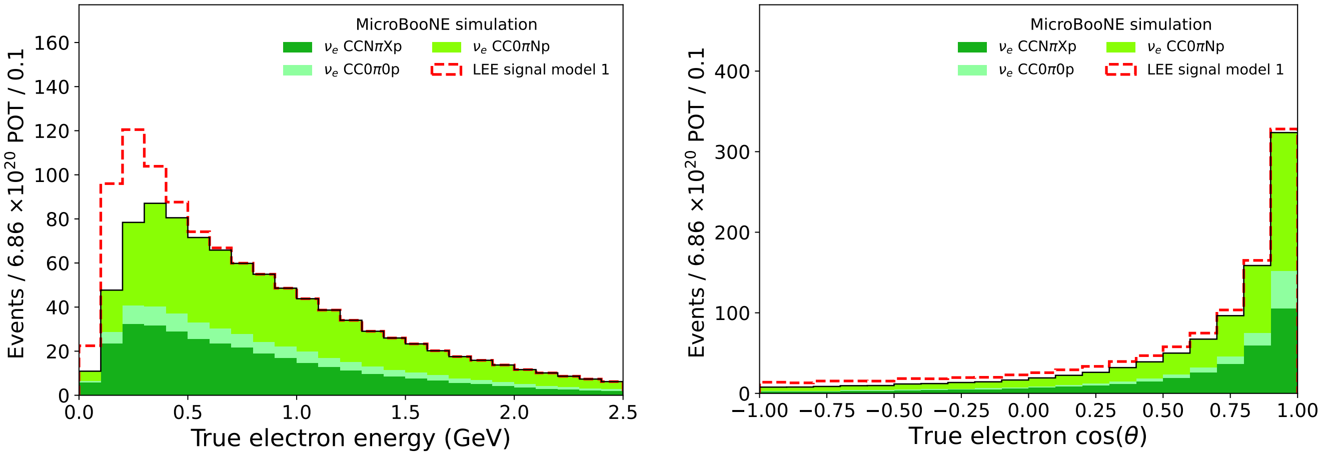


(a)

(b)

FIG. 8. The *LEE Signal Model 1* on MicroBooNE electron kinematics spectra in true $\nu_e$ events before any selection cuts are applied. The electron kinematics spectra are broken down into $\nu_e$ CC interactions with different numbers of final-state pions (0 or $N \geq 1$) and protons (0, $N$, or inclusive $X \geq 0$).

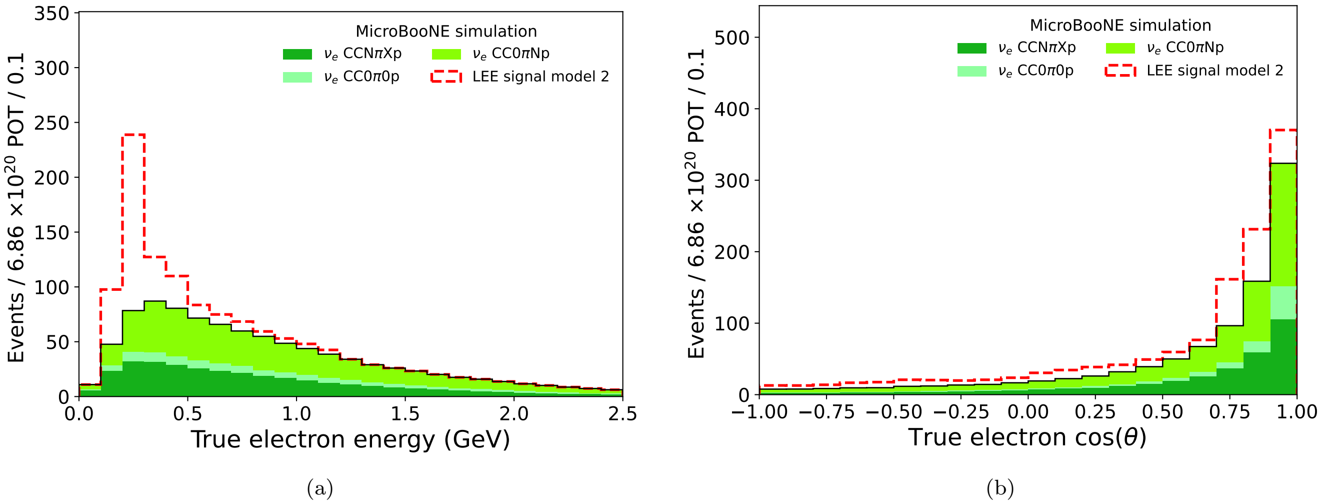


FIG. 9. The *LEE Signal Model 2* on MicroBooNE electron kinematics spectra in true $\nu_e$ events before any selection cuts are applied. The electron kinematics spectra are broken down into $\nu_e$ CC interactions with different numbers of final-state pions (0 or $N \geq 1$) and protons (0, $N$, or inclusive $X \geq 0$).

## V. EVENT RATES

Table I shows the table of predicted and observed event rates in the signal channels of this analysis. Total predictions are given with their systematic uncertainty. The $H_0$ predictions refer to the background-only hypothesis, while the $H_1$ predictions refer to the LEE hypothesis (under either signal model). The total prediction at the null hypothesis is furthermore broken down into its constituent event types.

| | Signal channel | |
|---|---|---|
| | $1e\mathrm{N}p0\pi$ | $1e0p0\pi$ |
| Data counts | 102 | 41 |
| Total $H_0$ prediction (constrained) | 133.5 ± 7.4 | 47.6 ± 3.7 |
| Total $H_1$ prediction (constrained, signal model 1) | 151.7 ± 8.2 | 55.3 ± 3.9 |
| Total $H_1$ prediction (constrained, signal model 2) | 168.5 ± 9.3 | 57.7 ± 4.1 |
| Total $H_0$ prediction (unconstrained) | 123.6 ± 17.1 | 42.8 ± 7.6 |
| Cosmics (unconstrained) | 0.8 | 5.3 |
| $\nu_e$ CC (unconstrained) | 104.1 | 18.4 |
| $\nu$ other (unconstrained) | 6.8 | 6.1 |
| $\nu$ NC $\pi^0$ (unconstrained) | 11.9 | 13.1 |
| MiniBooNE LEE Signal Model 1 (unconstrained) | 13.4 | 5.0 |
| MiniBooNE LEE Signal Model 2 (unconstrained) | 29.9 | 7.5 |

TABLE I. Predicted and observed event rates in the $1e\mathrm{N}p0\pi$ and $1e0p0\pi$ signal channels for events with a reconstructed energy of up to 1.55 GeV. Total predictions include MC and cosmic background and are given with systematic uncertainties.

## VI. TWO-HYPOTHESIS TESTS

This section shows the results of the two-hypothesis tests performed in the analysis. Several tests are performed to test both *LEE Signal Model 1* (based on unfolded neutrino energy, the same model used in the first iteration of this analysis [2]) as well as *LEE Signal Model 2* (built from the underlying shower kinematics). The tests are further repeated for the $1e\mathrm{N}p0\pi$ and $1e0p0\pi$ channels separately and combined. In Figs. 10 - 14, two curves are shown, representing the distribution of $\Delta\chi^2$ values obtained from toy experiments under the assumption that the null-hypothesis (no signal, $H_0$, in blue) is the underlying truth or that the signal model ($H_1$, in orange) represents the underlying truth. The vertical dashed line represents the median result for $H_1$ and is used to calculate the median sensitivity for ruling out the null hypothesis $H_0$ if the signal model hypothesis $H_1$ were true. The vertical solid line represents the observed $\Delta\chi^2$. The Bayes Factor (BF) is the probability density of the observed $\Delta\chi^2$ under $H_1$ divided by the probability density under $H_0$.

Fig. 10 shows two-hypothesis test results for the test of *LEE Signal Model 2* in the combined $1e\mathrm{N}p0\pi$ and $1e0p0\pi$ channels. The fit is performed in shower energy (Fig. 10a) and shower $\cos(\theta)$ (Fig. 10b). Fig. 11 shows expectations and results for a test of *LEE signal model 2* but now for the $1e\mathrm{N}p0\pi$ alone. Fig. 12 shows expectations and results for a test of *LEE signal model 2* but now for the $1e0p0\pi$ alone. Fig. 13 shows expectations and results for a test of *LEE signal model 1* for the two channels combined. Tests for *LEE signal model 1* for $1e\mathrm{N}p0\pi$ and $1e0p0\pi$ separately are shown in Fig. 14a and Fig. 14b, respectively.

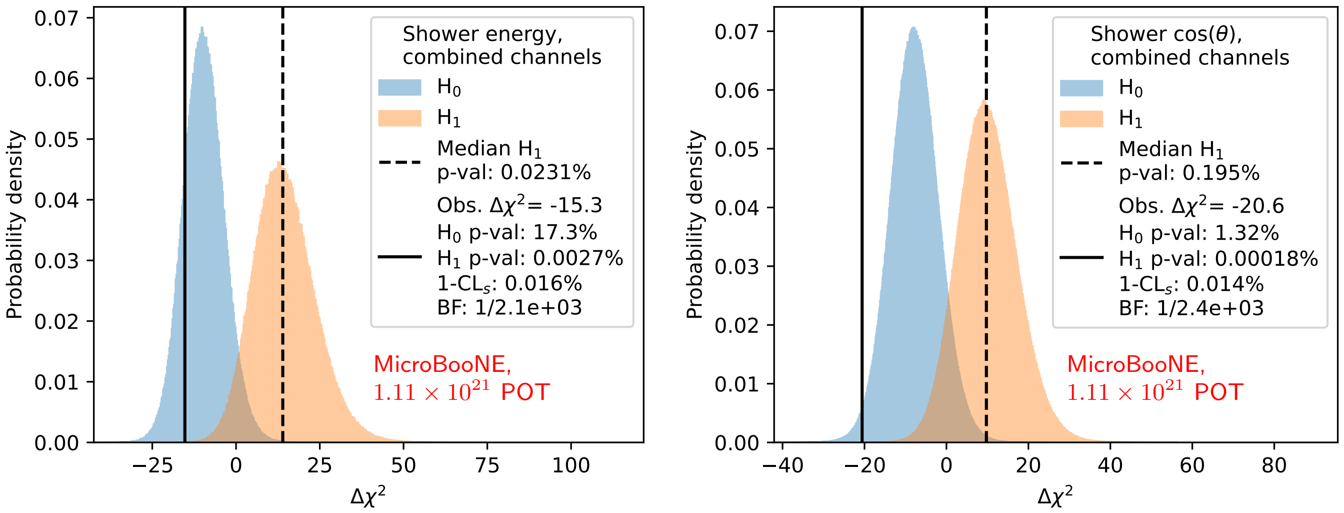


(a) (b)

FIG. 10. Two-hypothesis test using the *LEE Signal Model 2* based on shower kinematics binned in (a) shower energy and (b) $\cos(\theta)$, for the combined $1e\mathrm{N}p0\pi$ and $1e0p0\pi$ channels. The Bayes Factor (BF) is the probability density of the observed $\Delta\chi^2$ under $H_1$ divided by the probability density under $H_0$.

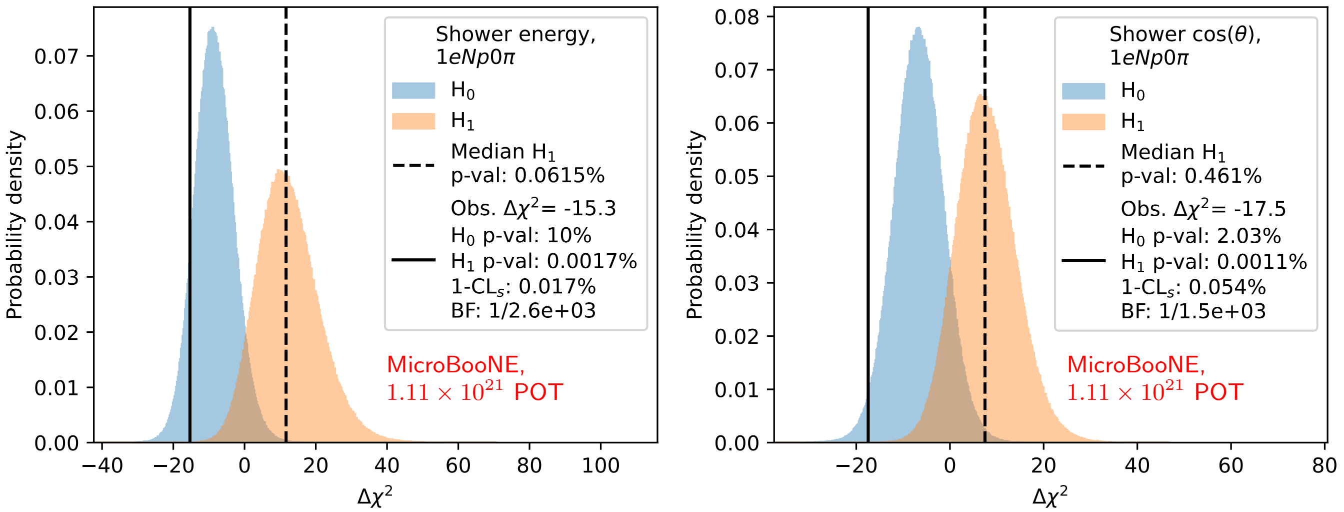


(a) (b)

FIG. 11. Two-hypothesis test using the *LEE Signal Model 2*, binned in shower kinematics (a: shower energy, b: shower $\cos(\theta)$), for the individual $1e\mathrm{N}p0\pi$ channel.

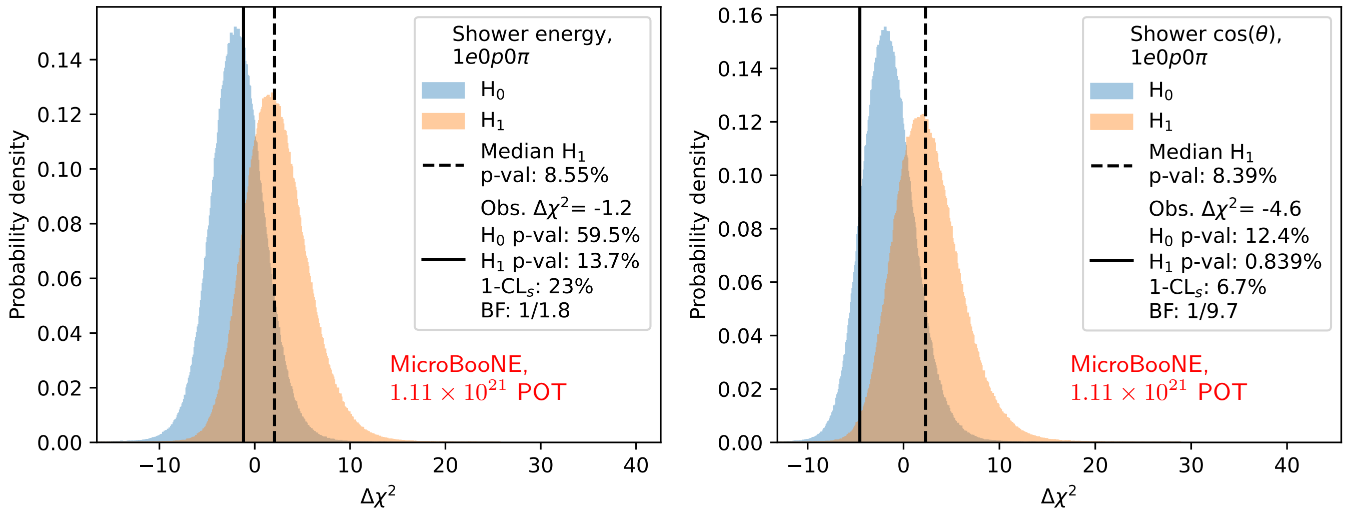


(a) (b)

FIG. 12. Two-hypothesis test using the *LEE Signal Model 2*, binned in shower kinematics (a: shower energy, b: shower $\cos(\theta)$), for the individual $1e0p0\pi$ channel.

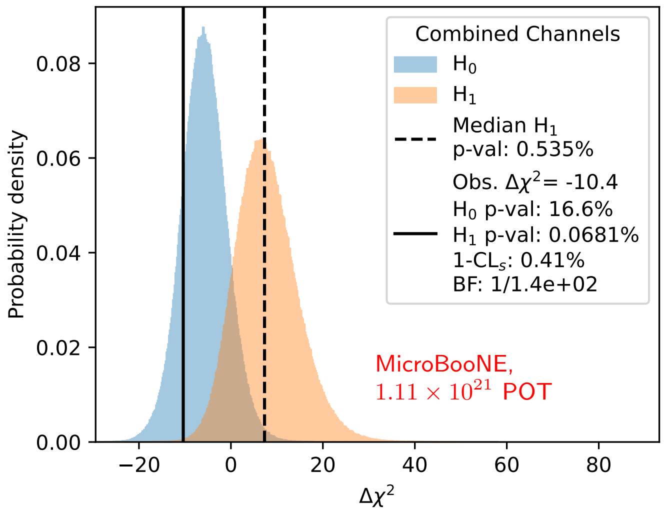


FIG. 13. Two-hypothesis test using the *LEE Signal Model 1*, binned in neutrino energy, for the combined $1e\text{N}p0\pi$ and $1e0p0\pi$ channels.

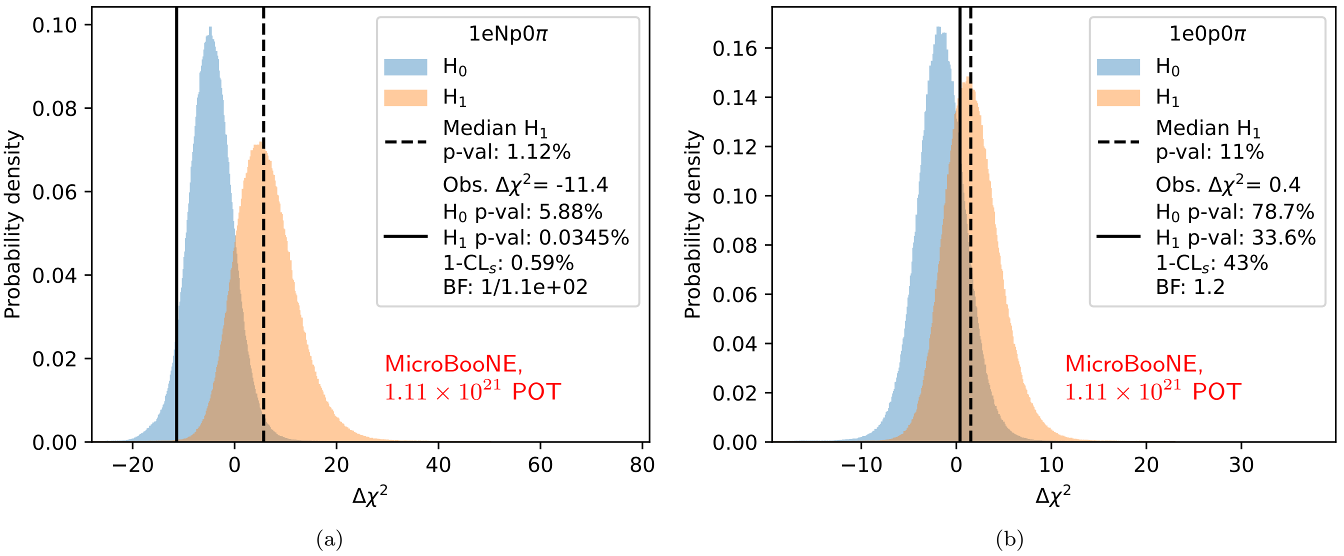


FIG. 14. Two-hypothesis test using the *LEE Signal Model 1*, binned in neutrino energy, for the individual signal channels (a: 1$e$N$p$0$\pi$, b: 1$e$0$p$0$\pi$).

## VII. SOURCES OF UNCERTAINTY

Figs. 15 - 17 show the contribution to the total systematic uncertainty in each histogram of the analysis. The uncertainties are shown as a fraction of the expectation value in each bin at the null-hypothesis. The error attributed to the prediction statistics includes the uncertainty due to limited MC statistics, as well as the statistical uncertainty on the cosmic background. Cross-section uncertainties include hadronic reinteraction effects.

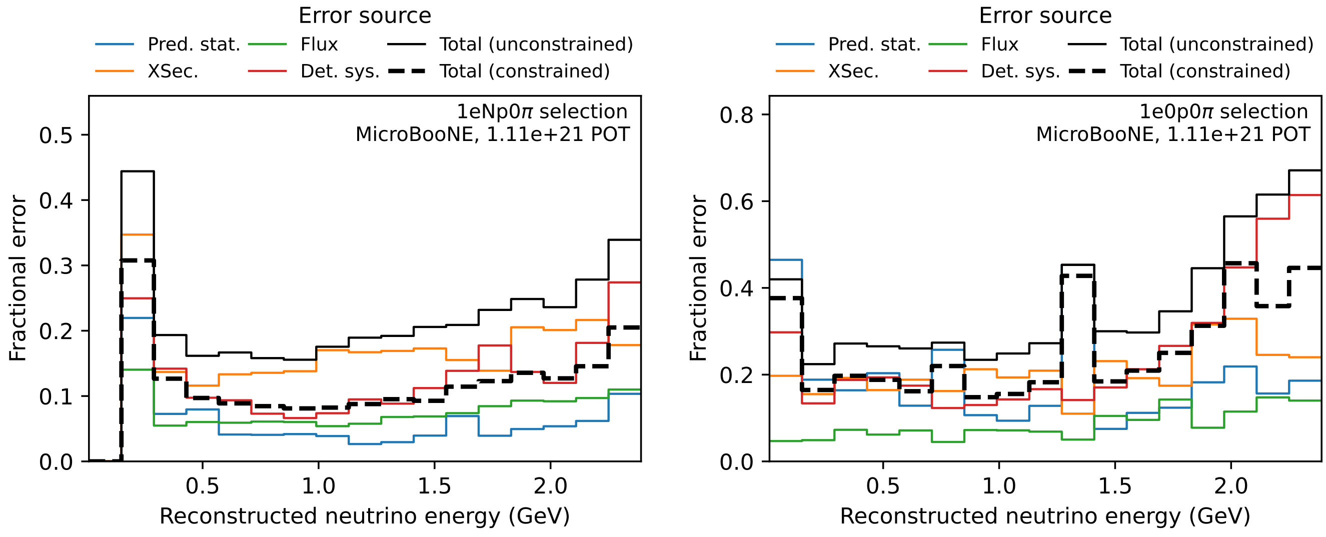


(a) (b)

FIG. 15. Fractional uncertainty in the signal channels binned in reconstructed neutrino energy (a: 1$e$N$p$0$\pi$, b: 1$e$0$p$0$\pi$).

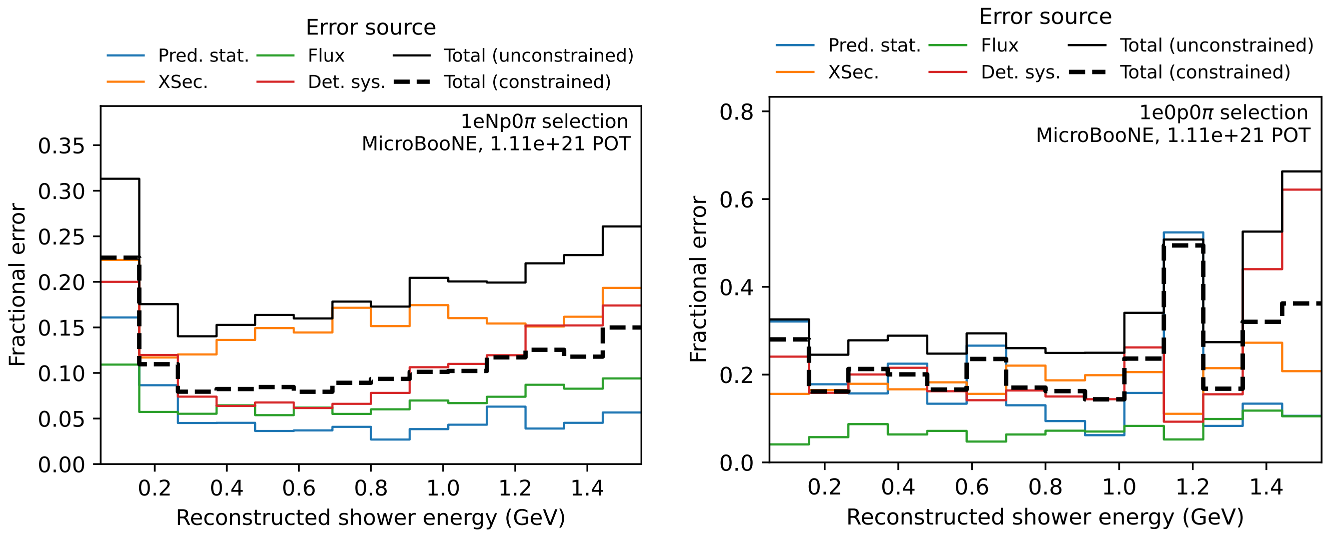


(a) (b)

FIG. 16. Fractional uncertainty in the signal channels binned in reconstructed shower energy (a: 1$e$N$p$0$\pi$, b: 1$e$0$p$0$\pi$).

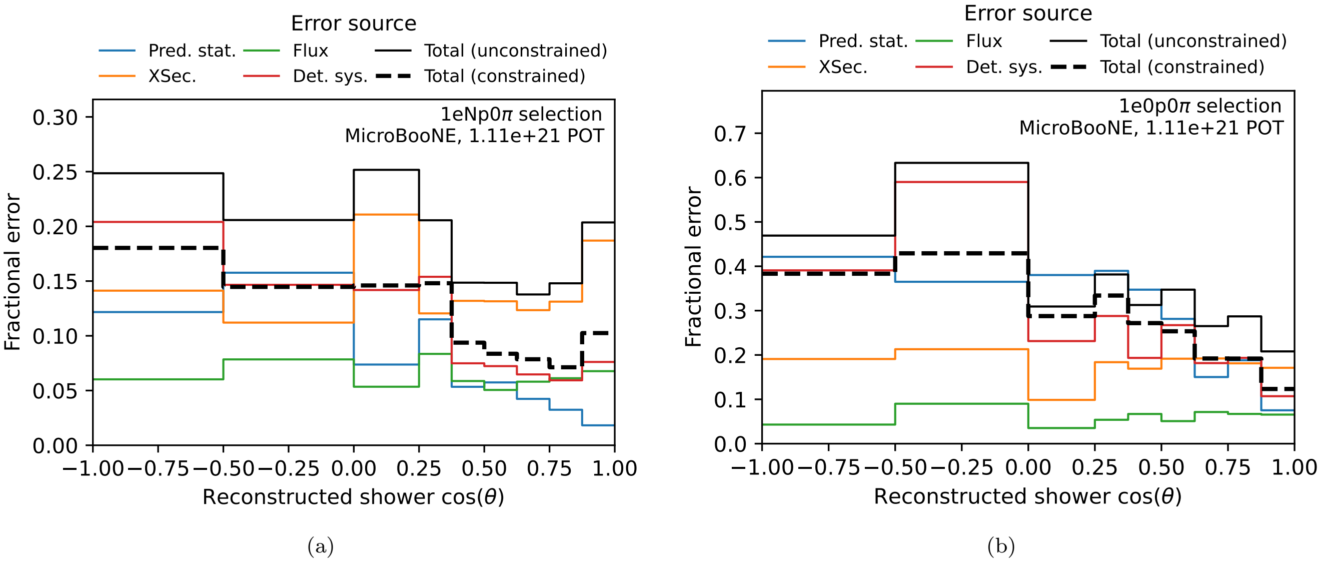


FIG. 17. Fractional uncertainty in the signal channels binned in reconstructed shower angle (a: $1e\mathrm{N}p0\pi$, b: $1e0p0\pi$).

## VIII. EVENT DISPLAYS

This section shows event displays of selected candidate events from the $1e0p0\pi$ (Fig 18) and $1e\mathrm{N}p0\pi$ (Fig. 19) selections.

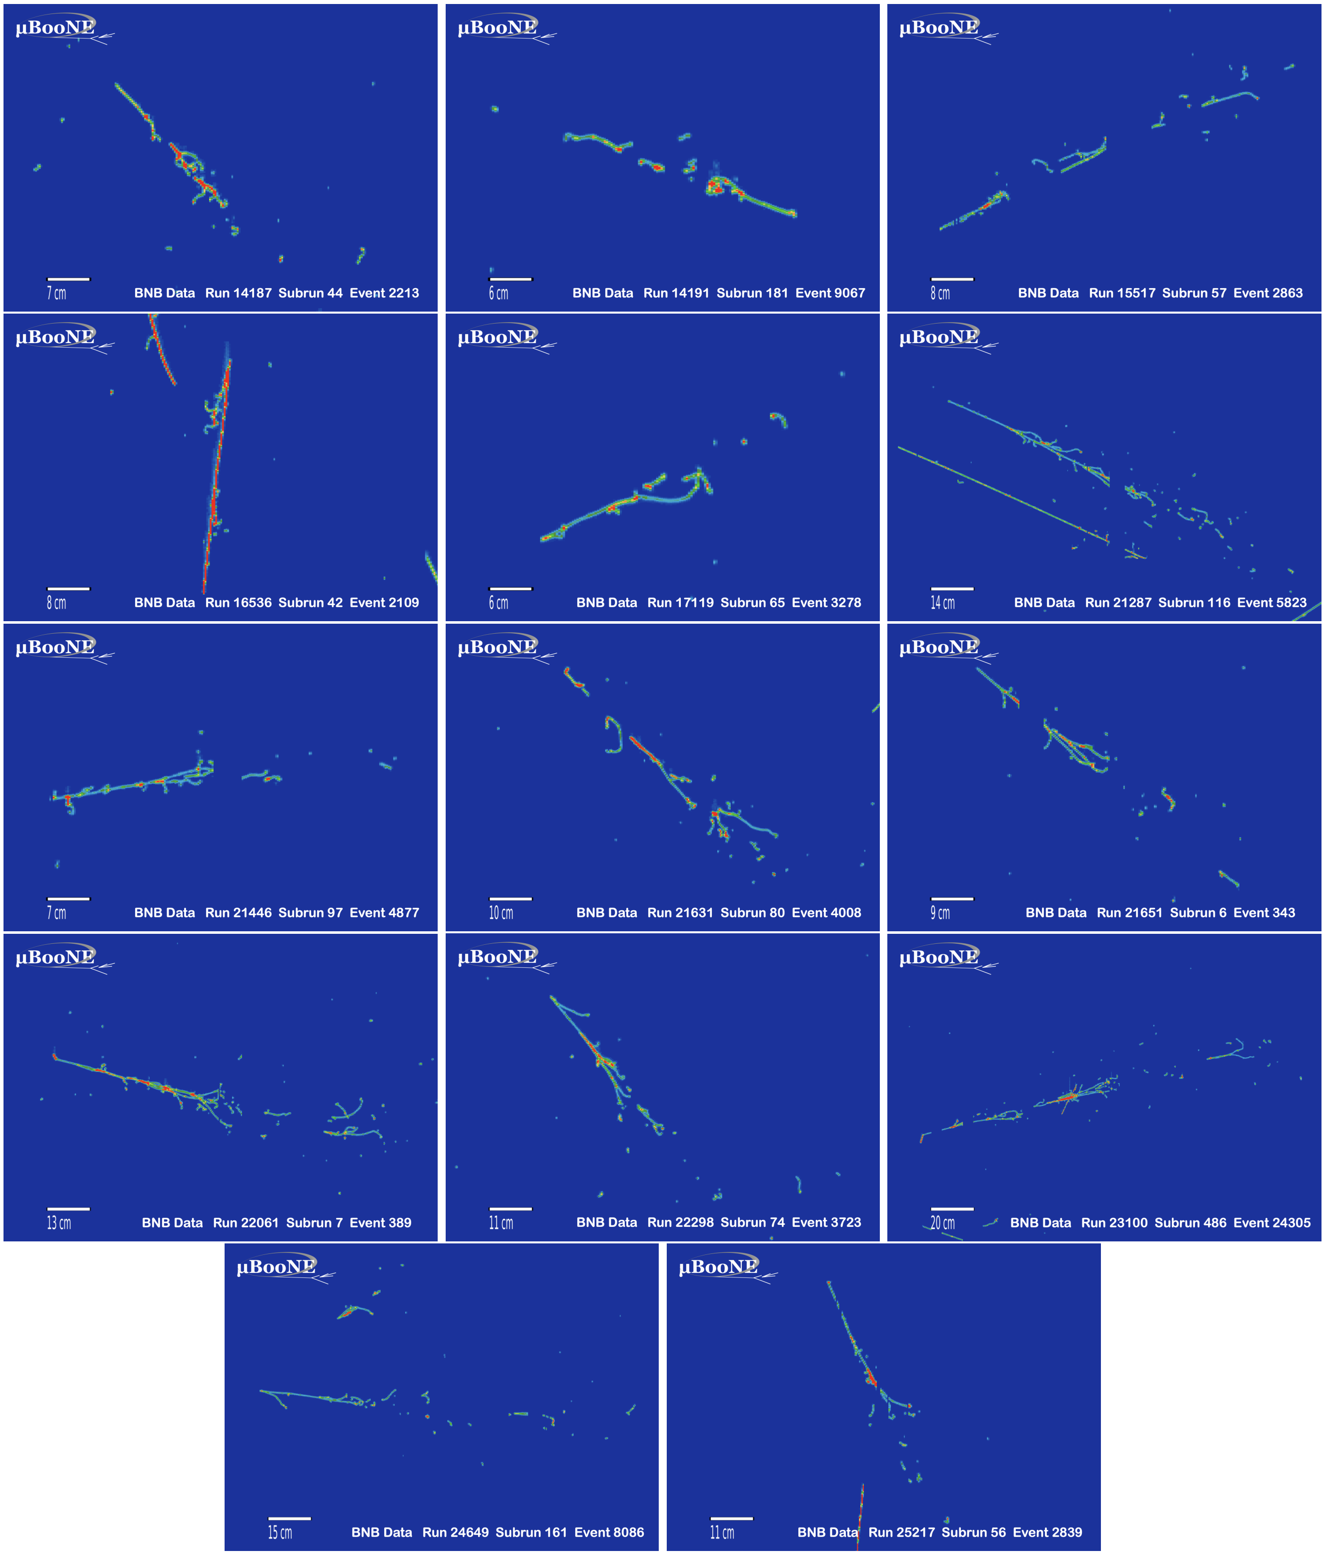


FIG. 18. Event displays of selected electron neutrino candidate data events in the $1e0p0\pi$ signal channel.

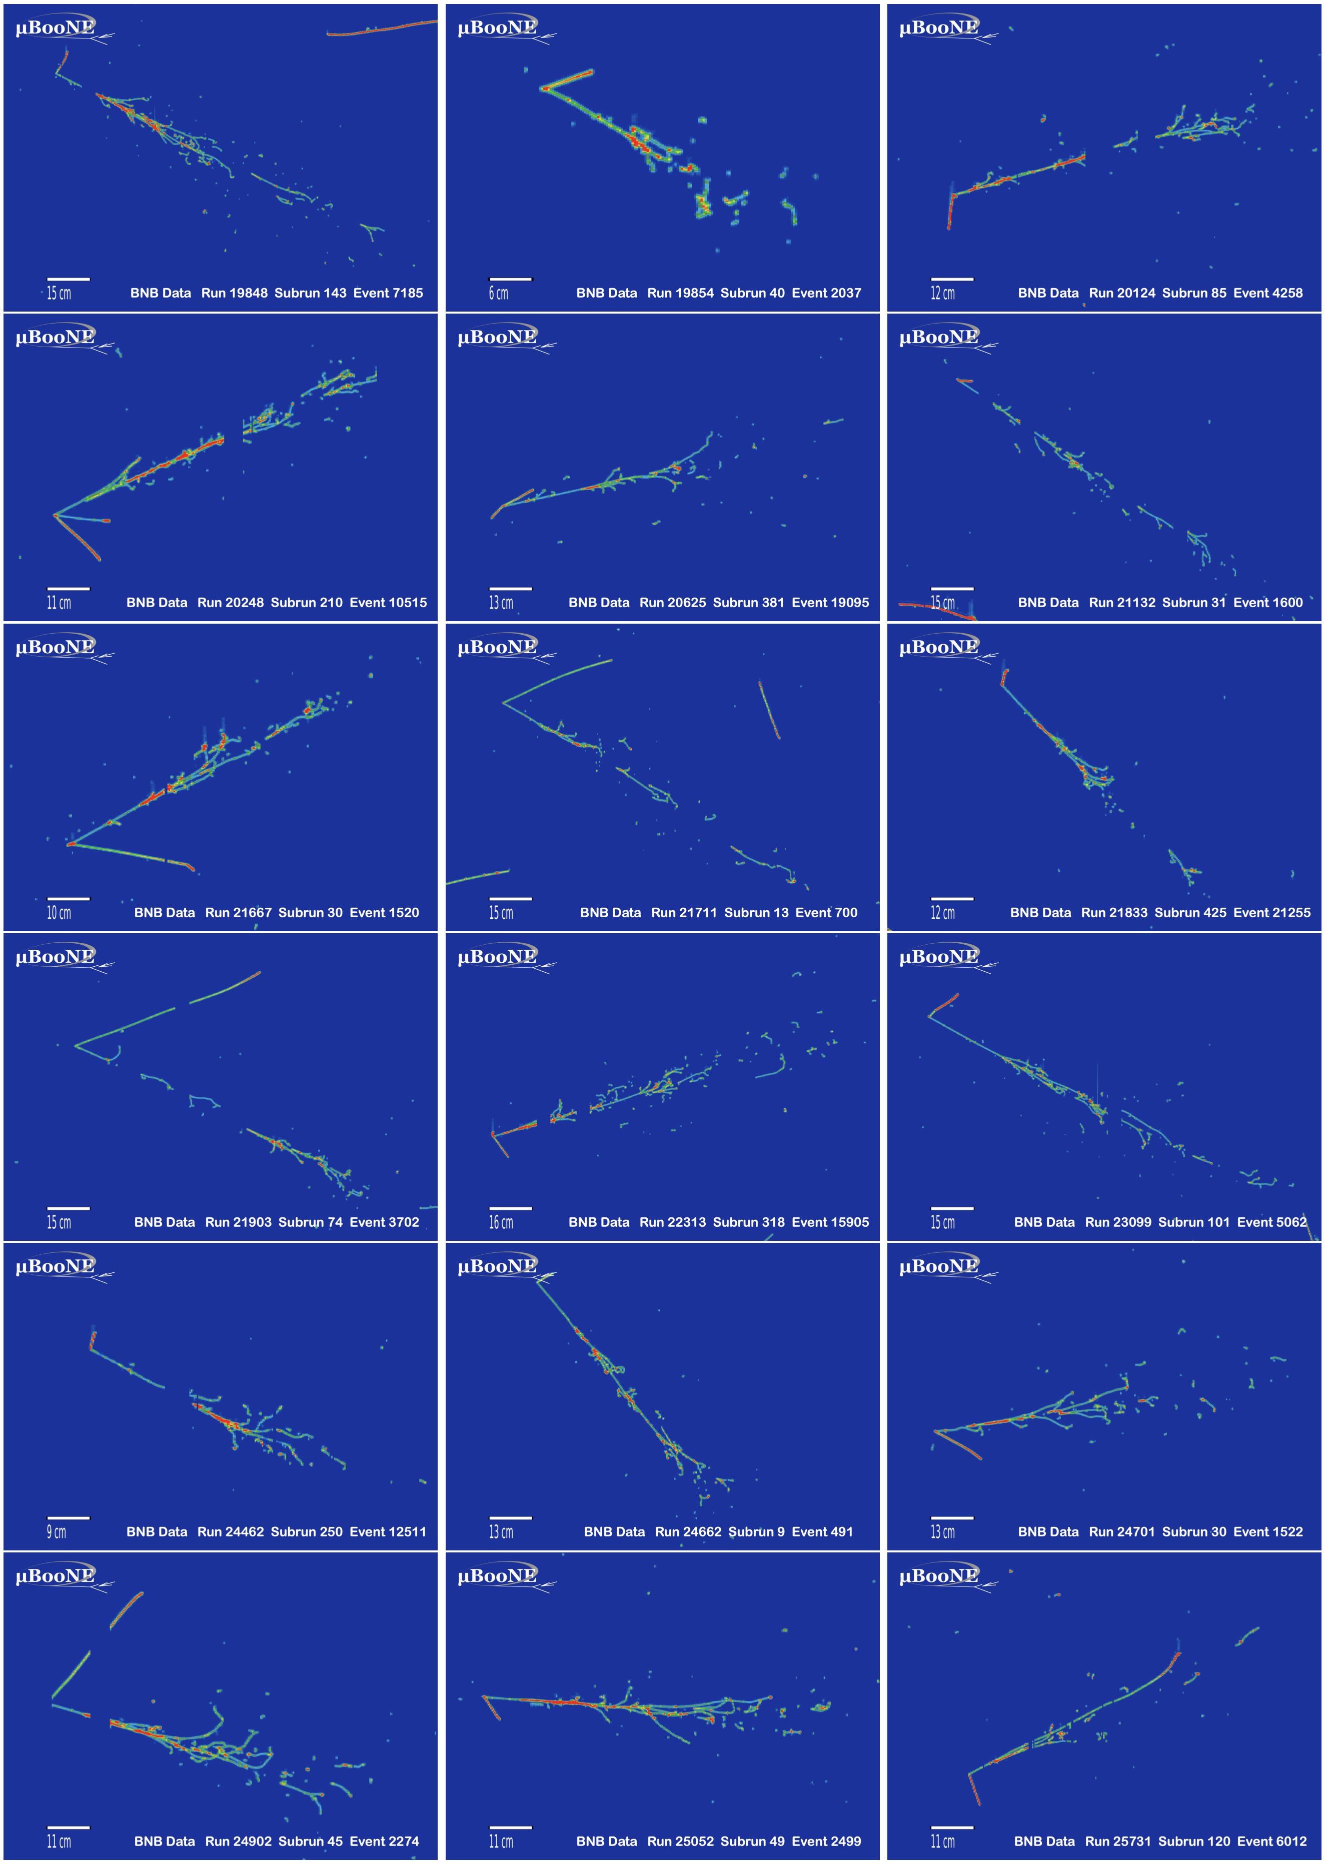


FIG. 19. Event displays of selected electron neutrino candidate data events in the $1eNp0\pi$ signal channel.

[1] C. Adams *et al.* (MicroBooNE Collaboration), J. Instrum. **14**, P04004 (2019).
[2] P. Abratenko *et al.* (MicroBooNE Collaboration), Phys. Rev. D **105**, 112004 (2022).
[3] MicroBooNE Collaboration, MICROBOONE-NOTE-1043-PUB, DOI:10.2172/1573217 (2018).
